# Supplementary material for: Hands Off my Database: Ransomware Detection in Databases through Dynamic Analysis of Query Sequences
Source: arXiv:1907.06775 source file (2019-07-15)
Supplement: Supplementary file 1 [file 99_appendix.tex]

\appendix

\section{Query Rewriting}\label{sec:appendix_rewriting}

Table~\ref{tab:appendix_rewriting} shows the commands that are rewritten when using the query rewriter.

\begin{table*}
    \centering
    \begin{tabular}{| l | l |}
    \hline
    Command & {WHERE | AND} \\ \hline
    SHOW PLUGINS & no rewriting possible \\ \hline
    SHOW DATABASES &  `Database` NOT LIKE 'dimaqs\%'\\ \hline
    SHOW TABLES & rewriting not needed \\ \hline
    SHOW TRIGGERS & `Trigger` NOT LIKE 'dimaqs\%'\\ \hline
    SHOW COLUMNS & rewriting not needed\\ \hline
    SHOW VARIABLES & `Variable\_name` NOT LIKE 'dimaqs\%'\\ \hline
    SELECT FROM information\_schema.columns & SCHEMA\_NAME NOT LIKE 'dimaqs\%'\\ \hline
    SELECT FROM information\_schema.files & FILE\_NAME NOT LIKE './dimaqs\%'\\ \hline
    SELECT FROM information\_schema.key\_column\_usage & TABLE\_SCHEMA NOT LIKE 'dimaqs\%'\\ \hline
    SELECT FROM information\_schema.partitions & TABLE\_SCHEMA NOT LIKE 'dimaqs\%'\\ \hline
    SELECT FROM information\_schema.schemata & SCHEMA\_NAME NOT LIKE 'dimaqs\%'\\ \hline
    SELECT FROM information\_schema.tables & SCHEMA\_NAME NOT LIKE 'dimaqs\%'\\ \hline
    SELECT FROM mysql.db & Db NOT LIKE 'dimaqs\%'\\ \hline
    SELECT FROM performance\_schema.file\_instances & FILE\_NAME NOT LIKE '\%/dimaqs\%/'\\ \hline
    SELECT FROM performance\_schema.objects\_summary\_global\_by\_type & OBJECT\_SCHEMA NOT LIKE 'dimaqs\%'\\ \hline
    SELECT FROM performance\_schema.table\_handles & OBJECT\_SCHEMA NOT LIKE 'dimaqs\%'\\ \hline
    SELECT FROM performance\_schema.table\_io\_waits\_summary\_by\_index\_usage & OBJECT\_SCHEMA NOT LIKE 'dimaqs\%'\\ \hline
    SELECT FROM performance\_schema.table\_io\_waits\_summary\_by\_table & OBJECT\_SCHEMA NOT LIKE 'dimaqs\%'\\ \hline
    SELECT FROM performance\_schema.table\_lock\_waits\_summary\_by\_table & OBJECT\_SCHEMA NOT LIKE 'dimaqs\%'\\ \hline
    \end{tabular}
    \caption{Rewriting WHERE/AND}
    \label{tab:appendix_rewriting}
\end{table*}

\section{Post Evaluation Classifier States}\label{app:classifier}

Figure~\ref{fig:eval_classifier_bibspace} visualizes the state of the classifier Petri net after processing all queries inside the Bibspace query set, while Figure~\ref{fig:eval_classifier_wiki} performs the same task for the Mediawiki query set.

\begin{figure}[ht]
    \centering
    \input{figures/eval_classifier_bibspace.tex}
    \caption{State of the classifier Petri net after evaluation of the Bibspace query set. Large tokens with a number represent the same number of tokens, not colors.}
    \label{fig:eval_classifier_bibspace}
\end{figure}

\begin{figure}[ht]
    \centering
    \input{figures/eval_classifier_wiki.tex}
    \caption{State of the classifier Petri net after evaluation of the Bibspace query set. Large tokens with a number represent the same number of tokens, not colors.}
    \label{fig:eval_classifier_wiki}
\end{figure}
